# Supplementary material for: Gromov boundary of the Grand Arc graph
Source: arXiv:2607.00957 source file (2026-07-01)
Supplement: Supplementary file 2 [file Appendix.tex]

\section{Appendix}

Here's a list of things Arya thinks we can add at the end of our paper as an appendix.

\subsection{High-filling grand lines}

Throughout the paper, we restrict to the case when $\Sigma$ has at least 3 maximal end classes. The once-punctured Cantor tree is the other example when $\mathcal{G}(\Sigma)$ is hyperbolic. 

We should prove that our grand ending laminations correspond to the Bavard-Walker setup, and conjecture that we can realize the grand ending laminations as connected components of high-filling grand lines (up to an appropriate definition of grand lines). 

\subsection{Finite type case}

We should remark that our setup corresponds to the standard ending laminations setup for finite-type surfaces.

\subsection{Witnesses and such}

We should check Masur and Schleimer's axioms for witnesses regarding when we have hyperbolic combinatorial complexes, to try and generalise our arguments to those settings.

\subsection{Quasimorphisms etc}
Bavard-Walker second paper uses their ideas for high filling rays to talk about quasi-morphisms of the big mapping class group. Can we do this ourselves now?
